# Supplementary material for: Random Walks with Erasure: Diversifying Personalized Recommendations on Social and Information Networks
Source: arXiv:2102.09635 source file (2021-02-25)
Supplement: Supplementary file 1 [file 10_appendix.tex]

\vspace{-2mm}
\section{Appendix}
\label{sec:appendix}

\subsection{Implementation Details for RWE}
\label{sec:appendix_implementation}
The source code of our implementation is available at~\footnote{\url{http://anonymous}}.
We found that RWE starts to converge in $< 10$ iterations, but for uniformity all the results in Table~\ref{tab:summary_comparison} are from runs of ten iterations. We set $\epsilon = 0.1$~\footnote{We
leave the exploration of other $\epsilon$ values for future work.}.
For large datasets, random walk explorations of RWE can be easily parallelized, since walks from each user-node can start independently of others. 

\subsection{Optimization for Section~\ref{sec:ideology}}
\label{sec:appendix_optimization}
We can write the probability of a user endorsing a political-content using the logistic function,
\vspace{-1mm}
\begin{align}
\label{eq:prob_url}
p(\textbf{S}_{u,i}=1 \mid \theta_u, \psi_i, \alpha_u, \gamma_i) & = \frac{1}{exp(- \|\theta_u - \psi_i\|^2 + \alpha_u + \gamma_i)}
\end{align}
, where $\lambda_{i}$ is the bias term associated with $i$.

Using Bayesian inference and under the assumption that all observed endorsements $\textbf{R}_{u,e}$ are independent, we get the following:
\begin{align}
\label{eq:lk_retweet}
p(\theta, \phi, \alpha, \beta \mid \textbf{R}) \propto \prod_{(u,e)\in \mathcal{U}\times\mathcal{E}} & p(\textbf{R}_{u,e}=1 \mid \theta_u, \phi_e, \alpha_u, \beta_e)^{a_{u,e}} \\ \nonumber
& (1-p(\textbf{R}_{u,e}=1 \mid \theta_u, \phi_e, \alpha_u, \beta_e))^{1-a_{u,e}}
\end{align}
The parameter $a_{u,e}$ is used to assign confidence to the observed endorsement of $e$ by $u$, and it could be a function of the number of times $u$ has endorsed $e$. %

Similarly, by Bayesian inference and the assumption that all observed $\textbf{S}_{u,i}$'s are independent, we arrive the following expression:
\begin{align}
\label{eq:lk_url}
p(\theta, \psi, \alpha, \gamma \mid \textbf{S}) \propto \prod_{(u,i)\in \mathcal{U}\times\mathcal{I}} & p(\textbf{S}_{u,i}=1 \mid \theta_u, \psi_i, \alpha_u, \gamma_i)^{b_{u,i}} \\ \nonumber
& (1-p(\textbf{S}_{u,i}=1 \mid \theta_u, \psi_i, \alpha_u, \gamma_i))^{1-b_{u,i}}
\end{align}
The parameter $b_{u,i}$ is used to assign confidence to the observed endorsement of $i$ by $u$, for example the number of endorsements. %

To simplify the notation, 
we write $\Pi_{u,e} = - \|\theta_u - \phi_e\|^2 + \alpha_u + \beta_e$, and 
similarly for $\Pi_{u,i}$.

After placing standard normal priors on $\theta$, $\phi$, and $\psi$, and adding the contribution from elite-endorsement~\eqref{eq:lk_url} as an additional regularizer %
on~\eqref{eq:lk_retweet}, we get the following log-likelihood function for joint optimization, where the parameter $\mu$ trades-off the contribution from elite-endorsement graph:
\vspace{-2mm}
\begin{align}
\label{eq:lk_url_final}
\argmax_{\theta, \phi, \psi, \alpha, \beta, \gamma} \ & p(\theta, \phi, \psi, \alpha, \beta, \gamma \mid \textbf{R}, \textbf{S}) \propto \\ \nonumber
& \mu \sum_{(u,e)\in \mathcal{U}\times\mathcal{E}}
a_{u,e} (\Pi_{u,e}) - log (1 + exp(\Pi_{u,e})) - \\ \nonumber
& \sum_{(u,i)\in \mathcal{U}\times\mathcal{I}} 
b_{u,e} (\Pi_{u,i}) - log (1 + exp(\Pi_{u,i})) \\ \nonumber
& - \frac{\lambda}{2}\|\theta\|_2 - \frac{\lambda}{2}\|\phi\|_2 - \frac{\lambda}{2}\|\psi\|_2 
\end{align}

The local optima %
can be found via a gradient-based optimization in which all but one parameter are fixed at each step and they are updated alternatively.
